# Supplementary material for: Controlling the folding and substrate-binding of proteins using polymer brushes
Source: arXiv:1204.6177 source file (2012-04-27)
Supplement: Supplementary file 1 [file supplemental.pdf]

# Supplemental figures for "Controlling the folding and substrate-binding of proteins using polymer brushes"

Brenda M. Rubenstein, Ivan Coluzza and Mark A. Miller

March 2012

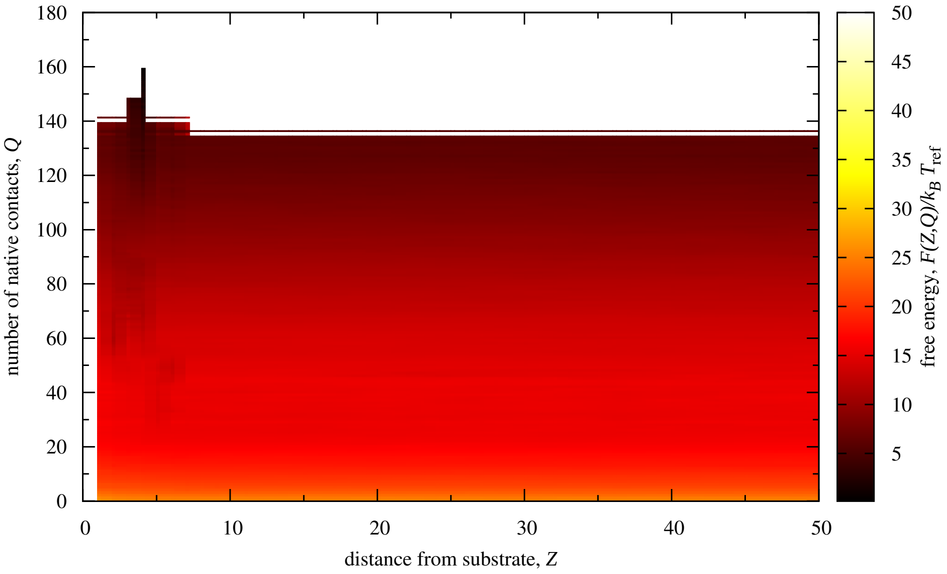


Figure 1: Free energy of protein 1 as a functon of both $Z$ (the distance from the substrate) and $Q$ (the total number of native contacts within the protein and between the protein and the substrate). The free energy decreases smoothly as the number of native contacts increases from $Q = 0$ to $Q = 136$ even for large $Z$, where the protein is out of range of the substrate. This indicates that the protein readily folds in solution. The narrow protrusion to the lowest free energy at $Z = 4$ corresponds to the folded protein slotting onto the substrate to obtain the remaining native contacts of the fully bound complex. The empty band at $Q = 135$ and $Q = 140$ reflects the underlying density of states of the lattice model; there are no states with precisely these numbers of native contacts for this particular protein and complex.

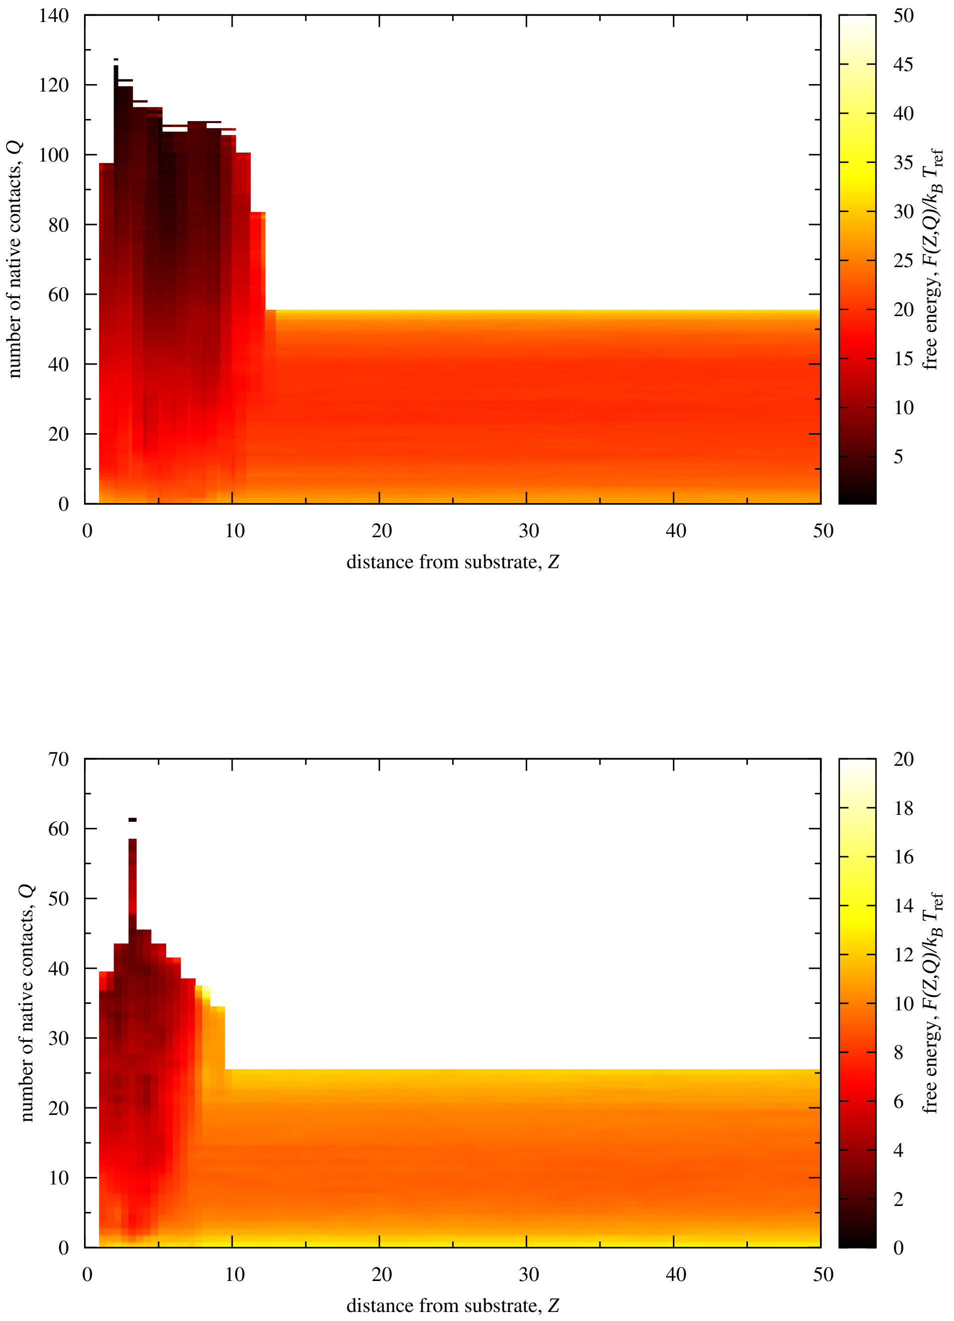


Figure 2: Equivalent of Figure 1 for proteins 2 (upper panel) and 3 (lower panel). In both cases there is no downhill gradient of the free energy with $Q$ when $Z$ is large, indicating that these proteins do not persistently adopt much of their native structure when out of range of the substrate. However, there is a decrease in the free energy when moving to low $Z$ at constant $Q$ (say, $Q = 40$ for protein 2 and $Q = 20$ for protein 3). The free energy can then be lowered to its minimum by increasing $Q$ when the protein is in contact with the substrate at low $Z$. This form of two dimensional energy is therefore characteristic of protein sequences that only form a thermodynamically stable folded structure in cooperation with binding to their substrates.
